# Supplementary material for: Phase function methods for second order linear ordinary differential equations with turning points
Source: arXiv:2209.14561 source file (2022-12-16)
Supplement: Supplementary file 1 [file appendix.tex]

%% \begin{section}{Appendix}

%% To see this, we observe that 
%% %% The function $F_\nu^\mu(x)$ defined for $-1 < x < 1$ via the formula 
%% %
%% \begin{equation}
%% \begin{aligned}
%% F_\nu^\mu(x) = 
%% &\sqrt{ \frac{2}{\pi}\ \frac{1}{\Gamma\left(\nu-\mu+1\right) \Gamma\left(\nu+\mu+1\right) } } 
%% \exp\left(-\frac{\pi}{2}\nu i\right)
%% \left(1-x^2\right)^{-\frac{\nu+1}{2}} \times \\
%% &\hskip 3em 
%% \int_0^\infty \exp\left(it \frac{x}{\sqrt{1-x^2}}\right) K_\mu(t) t^\nu\ dt,
%% \end{aligned}
%% \label{phase:alf:int}
%% \end{equation}
%% %
%% where $K_\nu(t)$ is the modified Bessel function of the third kind of order $\mu$,
%% satisfies the associated Legendre differential equation
%% %
%% \begin{equation}
%% (1-x^2) y''(x) - 2x y'(x) + \left(\nu(\nu+1) - \frac{\mu^2}{1-x^2}\right)y(x) = 0, \ \ -1 <x<1.
%% \end{equation}
%% %
%% %
%% The real and imaginary parts $u_\nu^\mu(x)$ and $v_\nu^\mu(x)$  of $F_\nu^\mu(x)$ are 
%% related to the usual Ferrer's functions $P_\nu^\mu$ and $Q_\nu^\mu$ of the first and second kinds 
%% (which are also sometimes referred to as the ``associated Legendre functions on the cut'') 
%% through the formulas
%% %
%% \begin{equation}
%% \begin{aligned}
%% %% F_\nu^\mu(x) = \exp\left( i \frac{3\pi}{2} \mu \right)
%% %% \left(Q_\nu^\mu(x) -\frac{\pi}{2} P_\nu^\mu(x)\right),\\
%% u_\nu^\mu(x) &= 
%% \sqrt{\frac{\pi}{2} \ \frac{\Gamma(\nu+\mu+1)}{\Gamma(\nu-\mu+1)}}
%% \left( 
%% \cos\left(\frac{\pi}{2} \mu \right)P_\nu^\mu(x) -\frac{2}{\pi} \sin\left(\frac{\pi}{2} \mu \right)Q_\nu^\mu(z)
%% \right)\ \ \mbox{and}
%% \\[1.3em]
%% v_\nu^\mu(x) &= 
%% \sqrt{\frac{\pi}{2} \ \frac{\Gamma(\nu+\mu+1)}{\Gamma(\nu-\mu+1)}}
%% \left( 
%% \sin\left(\frac{\pi}{2} \mu \right)P_\nu^\mu(x) + \frac{2}{\pi} \cos\left(\frac{\pi}{2} \mu \right)Q_\nu^\mu(z)
%% \right).
%% \end{aligned}
%% \end{equation}
%% %
%% The Wronskian of the pair $u_\nu^\mu, v_\nu^\mu$ is 
%% %
%% \begin{equation}
%% \omega(x) = \frac{1}{1-x^2},
%% \end{equation}
%% %
%% and when  $\mu=m$ is an integer, the $L^2$-normalized associated Legendre function 
%% of the first kind of order $\mu$ and degree $\nu$ is given by
%% %
%% \begin{equation}
%% \widetilde{P}_\nu^m(x) = (-1)^{m+1} \sqrt{\frac{2\nu+1}{\pi}} u_\nu^m(x).
%% \label{phase:alf:m}
%% \end{equation}
%% %
%% All of the preceding assertions follow easily from the material 
%% in Chapter~3 of \cite{HTFI}.


%% It follows from (\ref{phase:alf:int}) that the phase function $\alpha_{\nu,\mu}^{\mbox{\tiny alf}}$ corresponding
%% to the pair $u_\nu^\mu$, $v_\nu^\mu$, whose derivative is given by
%% %
%% \begin{equation}
%% \frac{d}{dx} \alpha_{\nu,\mu}^{\mbox{\tiny alf}}(x) = 
%% \frac{1}{1-x^2} \frac{1}{\left(u_\nu^\mu(x)\right)^2+\left(v_\nu^\mu(x)\right)^2},
%% \label{phase:alf:alphap}
%% \end{equation}
%% %
%% can be efficiently represented via
%% polynomial expansions, even when $\nu$ and $\mu$ are of large magnitude.
%% To see this, we first let 
%% %
%% \begin{equation}
%% x = \frac{w}{\sqrt{1+w^2}}
%% \end{equation}
%% %
%% in (\ref{phase:alf:int}) to obtain
%% %
%% \begin{equation}
%% \begin{aligned}
%% F_\nu^\mu\left(\frac{w}{\sqrt{1+w^2}}\right) = 
%% &\sqrt{ \frac{2}{\pi}\ \frac{\left(1+w^2\right)^{\nu+1}}{\Gamma\left(\nu-\mu+1\right) \Gamma\left(\nu+\mu+1\right) } } 
%% \exp\left(-\frac{\pi}{2}\nu i\right)
%% \int_0^\infty \exp\left(itw\right) K_\mu(t) t^\nu\ dt.
%% \end{aligned}
%% \label{phase:alf:int2}
%% \end{equation}
%% %
%% Next, we observe that 
%% %
%% \begin{equation}
%% \begin{aligned}
%% \left(u_\nu^\mu\left(\frac{w}{\sqrt{1+w^2}}\right)\right)^2
%% &+\left(v_\nu^\mu\left(\frac{w}{\sqrt{1+w^2}}\right)\right)^2
%% = 
%%  \frac{2}{\pi}\ \frac{(1+w^2)^{\nu+1}}{\Gamma\left(\nu-\mu+1\right) \Gamma\left(\nu+\mu+1\right) } \times \\
%% &\int_{-\infty}^\infty \exp(itw) G(t)\ dt,
%% \end{aligned}
%% \label{phase:alf:mod}
%% \end{equation}
%% %
%% where
%% %
%% \begin{equation}
%% G(t) =   \int_{\max(0,-t)}^\infty K_\mu(t+s) (t+s)^\nu K_\mu(s) s^\nu\ ds.
%% \label{phase:alf:convo}
%% \end{equation}
%% %
%% Since
%% %
%% \begin{equation}
%% K_\mu(z) \sim \sqrt{\frac{\pi}{2z}}\exp(-z)\ \ \mbox{as} \ \ z \to \infty,
%% \end{equation}
%% %
%% the function $K_\mu(t) t^\nu$ behaves similarly to a bump function centered
%% at the point $\nu+1/2$ when $\nu$ is of large magnitude.  It follows that the function $G$ defined in (\ref{phase:alf:convo})
%% resembles a bump function centered around the point $0$, again assuming $\nu$ is of large magnitude.
%% In particular, after a suitable change of variables,
%% %% From this together with (\ref{phase:alf:mod}) and (\ref{phase:alf:alphap}), we see that 
%% the phase function $\alpha_{\nu,\mu}^{\mbox{\tiny alf}}$ is the product of a polynomial and 
%% a function whose Fourier transform resembles a rapidly decaying bump function centered at $0$.
%% %% and can be efficiently represent via polynomial expansions, even  for large values of $\nu$ amd $\mu$.
%% Figure~\ref{phase:figure:1} contains plots of the functions $1/\Gamma(\nu) K_\mu(t) t^\nu$
%% and $1/\Gamma(\nu)^2 G(t)$.  


%% %% \begin{figure}[!h]
%% %% \hfil
%% %% \includegraphics[width=.45\textwidth]{alff.pdf}
%% %% \hfil
%% %% \includegraphics[width=.45\textwidth]{alfg.pdf}
%% %% \hfil
%% %% \caption{On the left is a plot of the function $1/\Gamma(\nu) K_\mu(t) t^\nu$ when $\nu=100$ and $\mu=20$.
%% %% On the right is a plot of $1/\Gamma(\nu)^2 G(t)$, where  $G$ is the function defined  in (\ref{phase:alf:convo}),
%% %% when $\nu=100$ and $\mu=20$.}
%% %% \label{phase:figure:1}
%% %% \end{figure}

%% %% \begin{equation}
%% %% f_{\nu,\mu}^{\mbox{\tiny alf}}(t) = 
%% %% \widetilde{P}_\nu^\mu(\tanh(w)) + 
%% %% \frac{2}{\pi} i \widetilde{Q}_\nu^\mu(\tanh(w))
%% %% \end{equation}
%% %% In each experiment, we fixed a value of $\mu$, sampled $m=200$ equispaced points
%% %% $x_1,\ldots,x_m$ in $[0,6]$ and constructed phase functions
%% %% $\alpha_{\nu,$
%% \end{section}
